# Supplementary material for: In-plane magnetocrystalline anisotropy in the van der Waals antiferromagnet FePSe$_3$ probed by magneto-Raman scattering
Source: arXiv:2307.12692 source file (2023-07-24)
Supplement: Supplementary file 1 [file FePSe3_Magnon_polaron_SM.pdf]

# Supplementary Materials for "In-plane magnetocrystalline anisotropy in the van der Waals antiferromagnet $FePSe_3$ probed by magneto-Raman scattering"

Dipankar Jana,[1,*] Piotr Kapuscinski,[1] Amit Pawbake,[1] Anastasios Papavasileiou,[2] Zdenek Sofer,[2] Ivan Breslavetz,[1] Milan Orlita,[1,3] Marek Potemski,[1,4,†] and Clement Faugeras[1,‡]

[1]*Laboratoire National des Champs Magnétiques Intenses, LNCMI-EMFL, CNRS UPR3228, Univ. Grenoble Alpes, Univ. Toulouse, Univ. Toulouse 3, INSA-T, Grenoble and Toulouse, France*
[2]*Chemistry Department, University of Chemistry and Technology Prague, 16628 Prague, Czech Republic*
[3]*Institute of Physics, Charles University, Ke Karlovu 5, Prague, 121 16, Czech Republic*
[4]*CENTERA Labs, Institute of High Pressure Physics, PAS, 01 - 142 Warsaw, Poland*

## I. SIMULATION FOR THE MAGNETIC FIELD DEPENDENCE OF MAGNON-PHONON COUPLED MODES: OTHER POSSIBILITIES

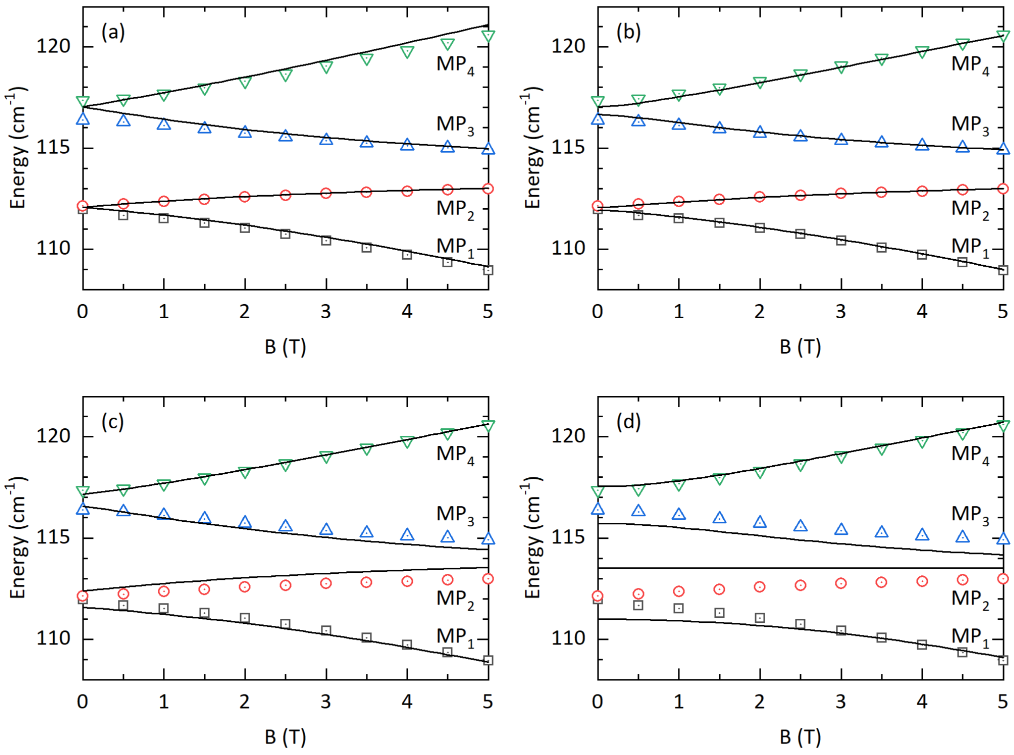


FIG. S1. Simulations to explore the magnetic field dependence of magnon-phonon coupled modes under different coupling scenarios: (a) selective coupling among degenerate $P_4$ modes and degenerate $M_{1,2}$ modes, excluding the coupling with $P_5$ and $P_6$ modes, (b) selective coupling among degenerate $P_4$ modes and degenerate $M_{1,2}$ modes, including the coupling with $P_5$ and $P_6$ modes, (c) selective coupling among non-degenerate $P_4$ modes and degenerate $M_{1,2}$ modes, and (d) Nonselective coupling among all the degenerate $P_4$ modes and degenerate $M_{1,2}$ modes. In Fig.S1a, we observe that the selective coupling among the degenerate coupled modes does not create any apparent splitting among the modes. The inclusion of coupling with $P_5$ and $P_6$ phonon modes (Fig.S1b) generates an apparent splitting that is small. Simulation with non-degenerate phonon modes (Fig.S1c) to match the apparent zero-field gap deviates largely from the experimental data at higher fields. Simulation with non-selective coupling (Fig.S1d) exhibited even greater deviation from the experimental outcome. Please note that in Fig.Sb-d, we considered the coupling with the $P_5$ and $P_6$ phonon modes, even though it was not explicitly shown.

* dipankar.jana@lncmi.cnrs.fr
† marek.potemski@lncmi.cnrs.fr
‡ clement.faugeras@lncmi.cnrs.fr

## II. LINEAR POLARIZATION-RESOLVED RAMAN SCATTERING

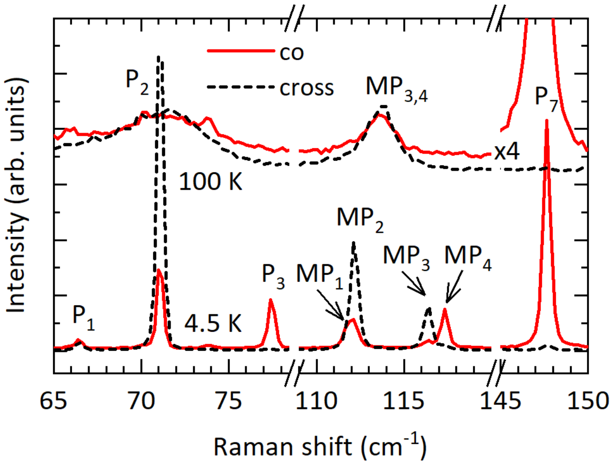


FIG. S2. Linear polarization-resolved Raman scattering spectra at two different temperatures, 4.5 K and 100 K. In Ref. 1 of the main script, the coupled modes were reported to exhibit circular polarization. However, our findings indicate that these modes at B=0 T also exhibit opposite linear polarization when excited with a linearly polarized laser. At 4.2 K, we estimate an apparent splitting of 0.15 $cm^{-1}$ between $MP_{1,2}$ and 0.9 $cm^{-1}$ between the $MP_{3,4}$ modes. The spectra at 100 K are scaled four times for better clarity. At this temperature, only the phonon modes ($MP_{3,4}$) are present among the coupled modes. Interestingly, we do not observe any splitting between $MP_{3,4}$ modes, which confirms the degeneracy of the bare phonons ($P_4$).

## III. SIMULATED SPLITTING BETWEEN THE PHONON-LIKE MODES ($MP_{2,3}$) AT 30 T

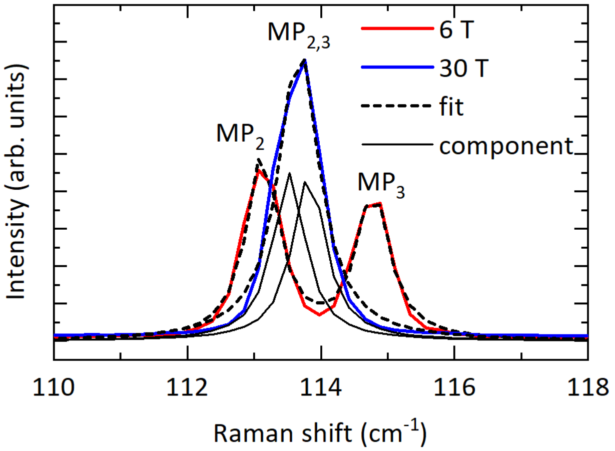


FIG. S3. Low-temperature Raman scattering spectra at 6 T and 30 T showing only the coupled modes $MP_{2,3}$. The well-separated peaks at 6 T are combined into a single peak at 30 T. We employed two Lorenzian peaks with equal widths to fit the modes at 6 T. To simulate these merged modes at 30 T, we constrain the width (0.3 $cm^{-1}$) of the peaks to be the same as that obtained at 6 T and the intensity to be the same for both modes. The peak energy of the two modes is treated as an adjustable parameter. Remarkably, a gap of 0.3 $cm^{-1}$ is estimated between the two components, aligning closely with the simulated field-dependent splitting (0.35 $cm^{-1}$) of $MP_{2,3}$ modes at 30 T. This confirms that the relatively larger splitting among the coupled modes at B=0 T is not due to the non-degeneracy of the phonon modes $P_4$.

## IV. TEMPERATURE DEPENDENT RAMAN SCATTERING IN WIDE ENERGY RANGE

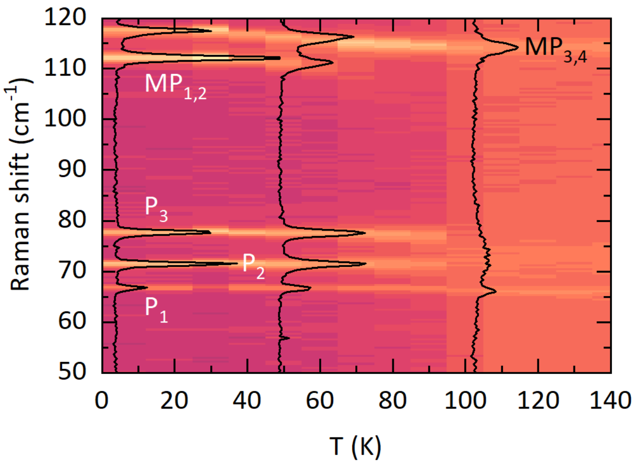


FIG. S4. False color map of the Raman scattering response of $FePSe_3$ as a function of temperature. The lowest energy peaks, labeled $P_{1,3}$, disappear when the temperature reaches Neel temperature ($T_N$) and are considered as phonons due to the folding of the Brillouin zone boundary onto the Γ point.
